# Supplementary material for: Query-Efficient Planning with Language Models
Source: arXiv:2412.06162 source file (2024-12-09)
Supplement: Supplementary file 1 [file 5_node_expansions.tex]

\begin{figure}
\begin{minipage}[b]{0.98\textwidth}
    \centering
    \includegraphics[width=\textwidth]{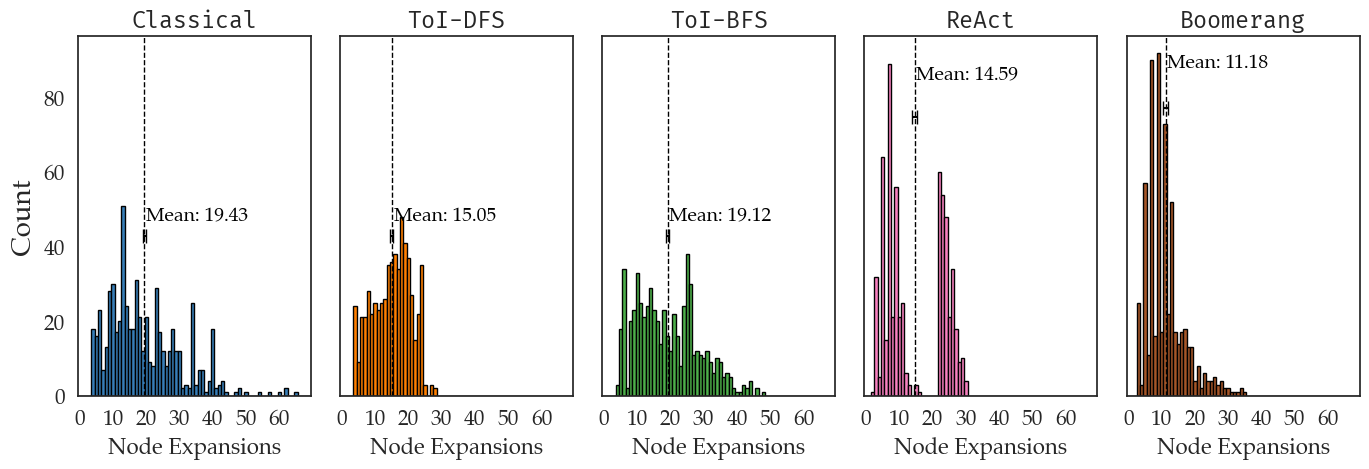}
    \caption{Histogram of interactive approaches' node expansions on Blocksworld problems. Count represents the number of runs that expanded a specific number of nodes (total of 600 runs). An idleness penalty causes the bimodalities between 20 and 30 expansions in the distribution.}
    \label{fig:ne_histogram}
\end{minipage}
\end{figure}

We report the corresponding node expansions in Fig.~\ref{fig:ne_histogram} to complement Fig.~\ref{fig:wmq_histogram}.

Among the LLM approaches, we observe that \boomerang{} is the most efficient with node expansions with a mean of 11.18. \react{} is the second most efficient but also suffers from the penalty discussed in Appendix~\ref{app:wmq_penalty}. \toidfs{} and \toibfs{} expand the most nodes compared to the other LLM approaches; however, they expand substantially less compared to their world model queries, or edge expansions, in Fig.~\ref{fig:wmq_histogram}. This is because the \toi{} methods in Blocksworld then to expand actions that undo state at each step which leads to many queries but not many more nodes expanded.

The classical planner \fd{} achieves 19.43 average expanded nodes. This is exactly 1 more than World Model Queries because it is an optimal planner.
