# Supplementary material for: Query-Efficient Planning with Language Models
Source: arXiv:2412.06162 source file (2024-12-09)
Supplement: Supplementary file 2 [file io_p_failure.tex]

\definecolor{lightgray}{gray}{0.9}
\definecolor{darkgray}{gray}{0.4}
\definecolor{purple}{rgb}{0.58,0,0.82}

% \lstdefinelanguage{plan}{
%   morekeywords={},
%   sensitive=true,
%   morecomment=[l]{//},
%   morestring=[r]"
% }

\lstset{
  language=plan,
  basicstyle=\ttfamily,
  keywordstyle=\color{blue},
  commentstyle=\color{darkgray},
  stringstyle=\color{purple},
  showstringspaces=false,
  columns=fullflexible,
  backgroundcolor=\color{lightgray},
  frame=single,
  breaklines=true,
  breakindent=0pt,
  postbreak=\mbox{{$\hookrightarrow$}\space},
  escapeinside={(*@}{@*)}
}

\begin{lstlisting}[basicstyle=\small]
------------ LLM Actions ------------
(unstack d a)
(put-down d)
(unstack a e)
(put-down a)
(unstack e c)
(stack e b)
------- LLM Predicted States ------
(clear a) (holding d) (on a e) (on c b) (on e c) (ontable b)
(clear a) (clear d) (handempty) (on a e) (on c b) (on e c) (ontable b) (ontable d)
(*@\aftergroup\speciallstcolor@*)(clear e) (holding a) (on c b) (on e c) (ontable b) (ontable d)(*@\aftergroup\endspeciallstcolor@*)
(clear a) (clear e) (handempty) (on c b) (on e c) (ontable a) (ontable b) (ontable d)
(clear c) (holding e) (on c b) (ontable a) (ontable b) (ontable d)
----------- Actual States ----------
(clear a) (holding d) (on a e) (on c b) (on e c) (ontable b)
(clear a) (clear d) (handempty) (on a e) (on c b) (on e c) (ontable b) (ontable d)
(*@\aftergroup\speciallstcolor@*)(clear d) (clear e) (holding a) (on c b) (on e c) (ontable b) (ontable d)(*@\aftergroup\endspeciallstcolor@*)
(clear a) (clear d) (clear e) (handempty) (on c b) (on e c) (ontable a) (ontable b) (ontable d)
(clear a) (clear c) (clear d) (holding e) (on c b) (ontable a) (ontable b) (ontable d)
\end{lstlisting}
