# Supplementary material for: Query-Efficient Planning with Language Models
Source: arXiv:2412.06162 source file (2024-12-09)
Supplement: Supplementary file 3 [file 12_why_20_wmq.tex]

The largest optimal plan length in Blocksworld (16) and Robotouille (18) are both under 20. These values informed our decision to limit \react{} to 20 steps and therefore the total number of world model queries (WMQ) to also be 20. We ablate the varying this 20 WMQ bound and observe the following:

\begin{table}[ht]
    \centering
    \begin{tabular}{lccccc}
        \toprule
        & \toibfs{} & \toidfs{} & \react{} & \classical{} & \boomerang \\
        \midrule
        16 & $0.21 \pm 0.017$ & $0.31 \pm 0.019$ & $0.52 \pm 0.020$ & $0.52 \pm 0.020$ & $0.80 \pm 0.016$ \\
        20 & $0.29 \pm 0.019$ & $0.40 \pm 0.020$ & $0.52 \pm 0.020$ & $0.63 \pm 0.020$ & $0.85 \pm 0.015$ \\
        24 & $0.35 \pm 0.019$ & $0.43 \pm 0.020$ & $0.52 \pm 0.020$ & $0.74 \pm 0.018$ & $0.86 \pm 0.014$ \\
        \bottomrule
    \end{tabular}
    \vspace{0.5em}
    \caption{Success of interactive LLM-based approaches when varying number of WMQ}
    \label{tab:multi-domain}
    \vspace{-1em}
\end{table}
