# Supplementary material for: Query-Efficient Planning with Language Models
Source: arXiv:2412.06162 source file (2024-12-09)
Supplement: Supplementary file 4 [file 6_penalty.tex]

One potential issue with world model queries is that approaches can look more efficient by terminating early or cycling between edges that have already been expanded. We address this by applying an "idleness" penalty which adds either 20 world model queries or node expansions to runs that expand fewer edges or nodes than the optimal number of edges or nodes to the goal. This can be interpreted as expanding the edges or nodes an approach would have expanded had it been acting optimally.
